# Supplementary material for: DE-PADA: Personalized Augmentation and Domain Adaptation for ECG Biometrics Across Physiological States
Source: arXiv:2502.04973 ancillary file (2025-02-07)
Supplement: Supplementary file 1 [file supplementary.pdf]

# Supplementary Material

## DE-PADA: Personalized Augmentation and Domain Adaptation for ECG Biometrics Across Physiological States

Amro Abu Saleh<sup>1</sup> 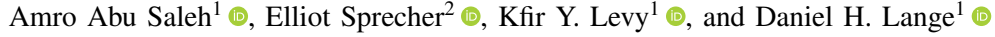, Elliot Sprecher<sup>2</sup> 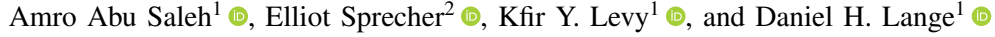, Kfir Y. Levy<sup>1</sup> 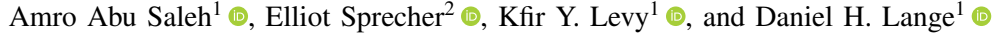, and Daniel H. Lange<sup>1</sup> 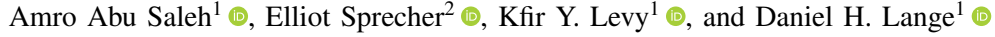

**Abstract**—This supplementary material outlines the methodology for identifying and excluding subjects with Electrocardiogram (ECG) patterns that significantly deviate from the majority population under resting and exercise conditions. Assuming that the majority represents normal physiological behavior, we employ Pearson correlation analysis, Fisher Z-transformation, and Gaussian Mixture Models (GMM) to detect statistical outliers whose ECG responses differ notably from the population.

### I. SUBJECTS WITH ATYPICAL ECG RESPONSE

#### A. Introduction

This chapter presents a comprehensive analysis of the correlation patterns between individual heartbeats and the median heartbeat under sitting posture and exercise conditions. The proposed method employs statistical techniques, including Pearson correlation, Fisher Z-transformation, and Gaussian Mixture Models (GMM), to identify subjects with atypical Electrocardiogram (ECG) patterns, including those exhibiting atypical changes exclusively during exercise. The objective is to retain only those subjects whose ECG patterns suggest they are likely healthy, while excluding subjects whose responses deviate significantly from the population.

It is important to note that this analysis does not diagnose or suggest the presence of any cardiac conditions, as such determinations require a specialist. Instead, we exclude subjects who may be suspected of having atypical or irregular patterns, based on statistical measures.

#### B. Correlation Analysis

We performed a Pearson correlation analysis to identify irregular ECG heartbeats. Since the heartbeats are aligned by R-peak location and the ECG is a semi-periodic signal, we expect similar segments (e.g., T-waves, P-waves) across different heartbeats to show high correlation due to their consistent characteristics.

Subjects marked in red in Fig. 1 and Fig. 2 were identified as outliers after completing the full analysis. They are marked throughout the analysis for illustrative purposes.

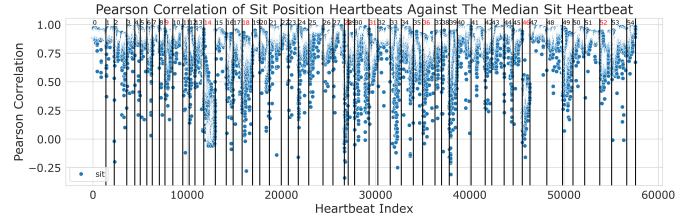

Fig. 1. Pearson correlation of all the heartbeats in sitting position with the median sit heartbeat, vertical lines separate between different subjects with the subjects' id in the top. Most subjects maintain high correlations with the median sit heartbeat, indicating relatively uniform patterns in a resting state. However, subjects 14, 28, and 46 show considerably lower correlations.

Fig. 1 displays the Pearson correlation coefficients of individual heartbeats recorded in the sitting position against the median heartbeat for that position across all subjects. Each point represents the correlation of a single heartbeat with the median heartbeat, providing insight into the alignment of each individual's heartbeat pattern with the average pattern for that position.

Most subjects maintain high correlations with the median sit heartbeat, indicating relatively uniform patterns in a resting state. However, a subset shows lower correlations, suggesting the presence of atypical ECG patterns even at rest. Fig. 2 presents the Pearson correlation coefficients of heartbeats for Exercise Phase 1 and Exercise Phase 2 compared to the median exercise heartbeat. The distribution reveals a broader range of correlations for exercise, suggesting that physiological changes induced by exercise affect the similarity between individual heartbeats and the median heartbeat pattern. We can observe that in addition to the subjects displaying low correlations in the sitting position, we have subjects displaying low correlations exclusively in exercise conditions.

#### Outliers Detection

In Fig. 3, we can observe a histogram of Pearson correlations of the heartbeats in exercise conditions. As expected it is concentrated with values close to 1 with a one-sided tail of lower correlations. We transform the Pearson correlation values into a Gaussian-like distribution using Fisher's Z-Transform [1], as shown in Fig. 4. This transformation normalizes the correlation values, making them suitable for

<sup>1</sup> Department of Electrical and Computer Engineering, Technion Israel Institute of Technology

<sup>2</sup> Independent Researcher.

Corresponding author: samro@campus.technion.ac.il

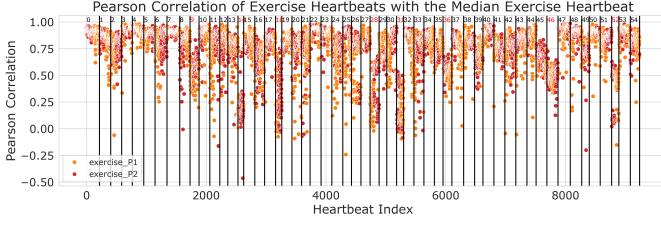

Fig. 2. Pearson correlation of all the heartbeats in exercise conditions with the median exercise heartbeat, vertical lines separate between different subjects with the subjects' id in the top. Most subjects maintain high correlations with the median exercise heartbeat, indicating relatively uniform patterns. However, in addition to the subjects in sitting positions, subjects 9, 18, 31, 36, and 52 show considerably lower correlations.

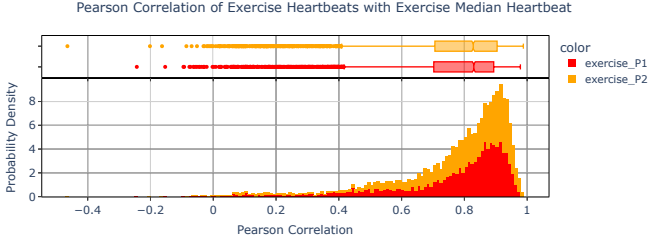

Fig. 3. The original distribution of Pearson correlation coefficients, indicating a concentration of high correlations with some potential outliers.

statistical analysis and enabling the detection of subjects with atypical ECG patterns. The Fisher Z-transformation is given by:

$$Z = \frac{1}{2} \ln \left( \frac{1+r}{1-r} \right) \quad (1)$$

where

$r$  Pearson correlation coefficient,  $r \in (-1, 1)$ .

In Fig. 4, the presented Gaussian-like distribution of transformed correlation values, as in most such distributions, the central portion consists of heartbeats with normal ECG patterns, and the somewhat long tails with what appear to be a large proportion of apparent statistical outliers. An alternative possibility is that we have a non-homogeneous population better characterized by a mixture distribution, that is, a mixture of more than one normal distribution.

Since the simple distribution is derived from correlation coefficients, these apparent outliers can be categorized into two groups, suggesting an overall mixture of 3 distributions:

- Right-side outliers: While heartbeats with high correlations could be mathematically categorized as outliers in a Gaussian distribution, they are not true outliers in the context of this analysis. Instead, these values represent individuals whose heartbeats exhibit exceptional consistency with the median heartbeat.
- Left-side outliers: These are the heartbeats considered true outliers, characterized by low correlations, representing individuals with atypical ECG patterns.

To distinguish these underlying populations, we perform a GMM analysis. GMM is a probabilistic model that effectively

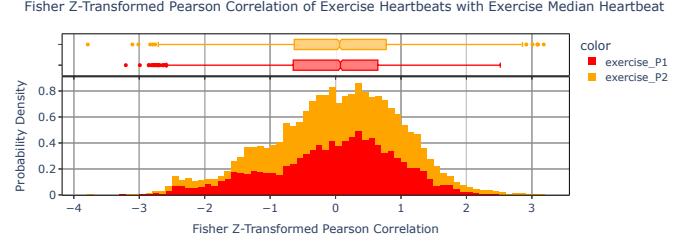

Fig. 4. Fisher's Z-Transformation effectively normalizes the data distribution, facilitating reliable statistical methods to detect subjects whose heartbeats significantly deviate from typical patterns.

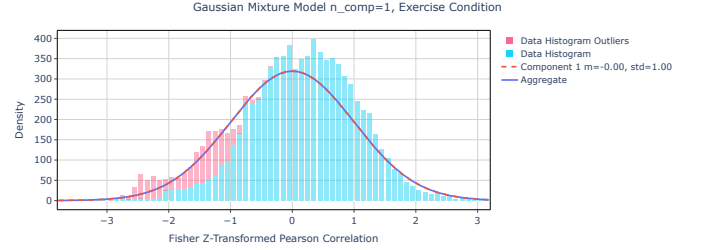

(a) GMM with 1 component.

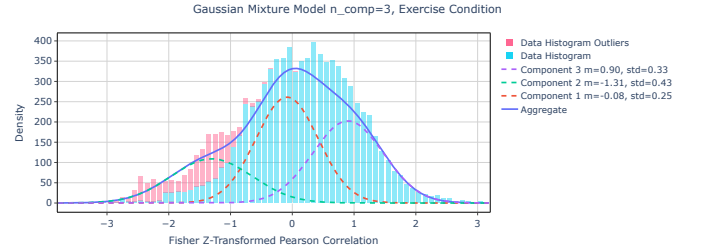

(b) GMM with 3 components.

Fig. 5. Gaussian Mixture Models with a different number of components.

captures the underlying distribution of data containing multiple subpopulations. Superiority of the fit of a derived mixture distribution can be demonstrated using various information statistics such as AIC [2] and BIC [3].

The GMM analysis was performed using models with 1 and 3 components to fit the Fisher Z-transformed Pearson correlations, as illustrated in Fig. 5. For the model with 1 component, the AIC and BIC values were 26,223 and 26,237, respectively, while the model with 3 components, yielded AIC and BIC values of 26,058 and 26,115. The lower AIC and BIC values observed for the 3-component model strongly suggest that it better captures the underlying structure of the data. In this model, one primary Gaussian represents the general population, while two additional components capture the tails of the distribution. Among these, the second Gaussian, which is shifted towards the left, identifies the outliers we aim to exclude from further analysis. This separation allows for a more accurate representation of the main population, supporting the use of the 3-component model for this purpose.

Our analysis so far has focused on individual heartbeats,

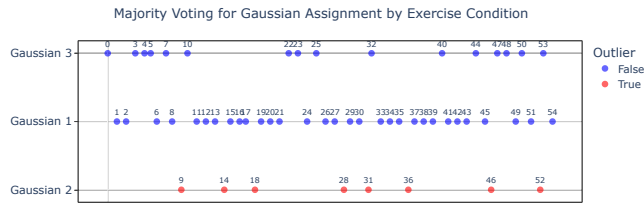

Fig. 6. Majority voting results with the subjects assigned to Gaussian 2 classified as outliers.

but our objective is to exclude entire subjects. To determine whether a subject should be classified as an outlier, we assign each heartbeat to its corresponding Gaussian component. The decision is made by majority voting: we count the number of heartbeats each subject has in each Gaussian, and the subject is assigned to the Gaussian with the majority of its heartbeats. We can see the assignment of the subjects to different Gaussian components in Fig. 6. The Gaussian component 2 contains 8 subjects which are classified as outliers and excluded from the database.

## REFERENCES

- [1] R. Fisher, *Statistical Methods for Research Workers*, ser. Biological monographs and manuals. Oliver and Boyd, 1970. [Online]. Available: <https://books.google.co.il/books?id=erPuAAAAMAAJ>
- [2] H. Akaike, "A new look at the statistical model identification," *IEEE Transactions on Automatic Control*, vol. 19, no. 6, pp. 716–723, 1974.
- [3] G. Schwarz, "Estimating the Dimension of a Model," *The Annals of Statistics*, vol. 6, no. 2, pp. 461 – 464, 1978. [Online]. Available: <https://doi.org/10.1214/aos/1176344136>
